# Supplementary material for: Learning Temporal Dependence from Time-Series Data with Latent Variables
Source: arXiv:1608.07636 source file (2016-08-27)
Supplement: Supplementary file 2 [file Appendix1.tex]

%\appendix

% \begin{center}
%  \Large{{\bf Appendix}}
% \end{center}
\section{Appendix: Proof of Theorem~\ref{thm:param}}\label{apx:ProofThm1} 

For our analysis, we use the equality $\mathsf{vec}(S_1RS_2)=(S_2^T  \otimes S_1)\mathsf{vec}(R)$ \cite{petersen2008matrix}, where $\mathsf{vec}$ is the vec-operator which stacks the columns of a matrix into a vector, $\otimes$ is the  Kronecker product, and $S_1$, $S_2$ and $R$ are square matrices with the same size. We denote $\mathsf{vec}(\Sigma_{(\cdot)})$ by $\mathsf{V}_{(\cdot)}$.
	
\begin{lem}\label{lm:zx}
	For every nonzero $i$, each entry of $\mathsf{V}_{ZX_{i}}$ can be written as a rational function, where both the nominator and the denominator are multivariate polynomials in entries of matrices $A$ and $B$, pmf $Q$, $\mathsf{V}_{V}$, $\mathsf{V}_{ZX_0}$ and $\mathsf{V}_{X_{j}}$ where $j\in [0,i-1]$ if $i> 0$ and $j\in [i,-1]$ if $i< 0$.
\end{lem}
\begin{proof}
	We have
	\begin{align}
	\mathsf{V}_{VX_{-i}}=&(A\otimes I)\mathsf{V}_{VZ_{\tau+1-i}}+(B\otimes I)\mathsf{V}_{VX_{\tau+1-i}} + \mathsf{V}_{VV_{\tau-i}}, i \geq 1,\label{Eq:eq1-vx}\\
	\mathsf{V}_{VZ_{-i}}=&(A\otimes I)\mathsf{V}_{VZ_{1-i}}+(B\otimes I)\mathsf{V}_{VX_{1-i}}, i \geq 1.\label{Eq:eq1-vz}
	\end{align}	
	Note that if $i \leq \tau$, then $\mathsf{V}_{VZ_{\tau+1-i}}=\mathsf{V}_{VX_{\tau+1-i}}=0$. Therefore, for  $\mathsf{V}_{VZ_{\tau+1-i}}$ or $\mathsf{V}_{VX_{\tau+1-i}}$ to be nonzero, the subscript must be in $[1-i,0]$, which is greater than $-i$. As a result, for every $i\geq 1$ and recursively using Equations \ref{Eq:eq1-vx} and \ref{Eq:eq1-vz}, each entry of $\mathsf{V}_{VX_{-i}}$ can be returned as a multivariate polynomial in the entries of $\mathsf{V}_{VX_{0}}$, $\mathsf{V}_{VZ_{0}}$, $\mathsf{V}_V$, $A$, $B$ and the pmf $Q$. Given that $\mathsf{V}_{VX_{0}}=q_0\mathsf{V}_{V}$, $\mathsf{V}_{VZ_{0}}=\mathsf{V}_{V}$, we can conclude that for every $i\geq 0$, each entry of $\mathsf{V}_{VX_{-i}}$ is a  multivariate polynomial in the entries of $\mathsf{V}_V$, $A$, $B$ and the pmf $Q$.
	
	Also, using the equations of the system \ref{Eq:Mod}, we get:
	\begin{align}
	\mathsf{V}_{ZX_i}=&(I\otimes A)\mathsf{V}_{ZX_{i-1}}+(I\otimes B)\mathsf{V}_{X_{i-1}}, i \geq 1,\label{Eq:eqzxi}\\
	\mathsf{V}_{ZX_{-i}}=&(I\otimes A)\mathsf{V}_{ZX_{-i-1}}+(I\otimes B)\mathsf{V}_{X_{-i-1}}+ \mathsf{V}_{VX_{-i}}, i \geq 0.\label{Eq:eqzx-i}
	\end{align}	
	By recursive use of Equ.~\ref{Eq:eqzxi}, for every $i\geq 1$, each entry of $\mathsf{V}_{ZX_{i}}$ can be written as a multivariate polynomials in entries of $\mathsf{V}_{X_{j-1}}, j\in [1,i]$, and $\mathsf{V}_{ZX_0}$.
	Similarly, by recursive use of Equ.~\ref{Eq:eqzx-i}, for every $i\geq 0$, each entry of $\mathsf{V}_{ZX_{-i-1}}$ can be written as a rational function $\frac{R_1}{R_2}$, where $R_1$ and $R_2$ are multivariate polynomials in entries of $\mathsf{V}_{X_{-j-1}}$ and $\mathsf{V}_{VX_{-i}}$ for $j\in [0,i]$, and $\mathsf{V}_{ZX_0}$. Given that $\mathsf{V}_{VX_{-i}}$ is also a multivariate polynomial, the proof is complete.
\end{proof}

\begin{lem}\label{lm:zx0}
	We can represent $\mathsf{V}_{ZX}$ as a rational function, where both the nominator and the denominator are multivariate polynomials in entries of matrices $A$ and $B$, $D$, pmf $Q$, $\mathsf{V}_{V}$, and $\mathsf{V}_{X_{i}}$ where $i\in [0,\tau_{\max}-1]$.		
\end{lem}
\begin{proof}
	From the first equation of the system \ref{Eq:Mod}, we get:
	\begin{align}
	\mathsf{V}_{Z_i}&=(I\otimes A)\mathsf{V}_{Z_{i-1}}+(I\otimes B)\mathsf{V}_{XZ_{i-1}}, i\geq 1.\label{Eq:zi}
	\end{align}
	Also, from the second equation, we can write:
	\begin{align}
	\mathsf{V}_{ZX}&=\mathsf{V}_{Z_{\tau}}+(D\otimes I)\mathsf{V}_{ZX_{1}}.\label{Eq:zx}
	\end{align}
	According to Lemma \ref{lm:zx}, for $i\geq 2$, each entry $\mathsf{V}_{ZX_{i-1}}$ can be written as a  multivariate polynomial in entries of matrices $A$ and $B$, pmf $Q$, $\mathsf{V}_{ZX_0}$ and $\mathsf{V}_{X_{j}}$ where $j\in [0,i-2]$. 
	Let $i\in [1,\tau_{\max}]$. Since $\mathsf{V}_{Z_{\tau}}=\sum_{k=0}^{\tau_{\max}}q_k\mathsf{V}_{Z_{k}}$, Equations \ref{Eq:zi} and \ref{Eq:zx} together from a linear system of $(\tau_{\max}+1)$ equations in variables in $\mathsf{V}_{ZX}$, $\mathsf{V}_{Z_i}$ and $\mathsf{V}_{X_k}, k\in [0,\tau_{\max}-1]$. Therefore, the proof is complete.
\end{proof}

\begin{lem}\label{lm:VX}
	For every $i$, $\mathsf{V}_{X_i}$ is a rational function, where both the nominator and the denominator are multivariate polynomials in entries of matrices $A$ and $B$, $D$, pmf $Q$, and $\mathsf{V}_{V}$ and $\mathsf{V}_{W}$.
\end{lem}
\begin{proof}
	From the second equation of the system \ref{Eq:Mod}, we get:
	\begin{align}
	\mathsf{V}_{X}&=\mathsf{V}_{ZX_{-\tau}}+(I\otimes D)\mathsf{V}_{X_{-1}}+\mathsf{V}_W,\label{Eq:eqx0}\\
	\mathsf{V}_{X_i}&=\mathsf{V}_{ZX_{i-\tau}}+(I\otimes D)\mathsf{V}_{X_{i-1}}.\label{Eq:eqxi}
	\end{align}
	
	Let $k\in [0,\tau_{\max}]$. We have $\mathsf{V}_{ZX_{k-\tau}}=\sum_{j=0}^{\tau_{\max}}q_j\mathsf{V}_{ZX_{k-j}}$ and $|k-j|\in [0,\tau_{\max}]$. Therefore, according to Lemma \ref{lm:zx} and \ref{lm:zx0}, for every $k\in [0,\tau_{\max}]$, each entry of $\mathsf{V}_{ZX_{k-\tau}}$ can be returned as a rational fnction where both the nominator and denominator are multivariate polynomials in entries of $A$, $B$, $Q$, $\Sigma_V$, and $\Sigma_{X_l}, l\in [0,\tau_{\max}]$.
	
	Let $i\in [1,\tau_{\max}]$. Equations \ref{Eq:eqx0} and \ref{Eq:eqxi} together from a linear system of $(\tau_{\max}+1)$ equations in $\mathsf{V}_{X_k}, k\in [0,\tau_{max}]$. Therefore, the proof is complete.
\end{proof}

Equation~\ref{Eq:opt2} can be written as
\begin{align}\label{Eq:opt3}
B^{-1}\Sigma_{X_{i+1}}= K_1\Sigma_{X_i} -K_2\Sigma_{X_{i-1}} + \sum_{j=0}^{\tau_{\max}}q_j\Sigma_{X_{i-j}}, i\geq \tau_{\max}.
\end{align}
By expanding Equ.~\ref{Eq:opt3}, we can write
\begin{align}\label{Eq:mat1}
\Sigma_{X_{i-\tau_{\max}}} = \frac{1}{q_{\tau_{\max}}}B^{-1}\Sigma_{X_{i+1}} -\frac{1}{q_{\tau_{\max}}}(q_0I+K_1)\Sigma_{X_i} - \frac{1}{q_{\tau_{\max}}}(q_1I - K_2)\Sigma_{X_{i-1}} - \frac{1}{q_{\tau_{\max}}}\sum_{j=2}^{\tau_{\max}-1}q_j\Sigma_{X_{i-j}}, i\geq \tau_{\max}.
\end{align}
Writing Equ.~\ref{Eq:mat1} For $i \in [\tau_{\max} \; ,\; 2\tau_{\max}]$, we have
\begin{align}\label{Eq:identif}
\begin{bmatrix}
\Sigma_{X_{0}} & \Sigma_{X_{1}} & \dots & \Sigma_{X_{\tau_{\max}}}
\end{bmatrix}=
\begin{bmatrix}
\frac{B^{-1}}{q_{\tau_{\max}}} & -\frac{q_0I+K_1}{q_{\tau_{\max}}} & - \frac{q_1I - K_2}{q_{\tau_{\max}}} & -\frac{q_2}{q_{\tau_{\max}}}I & -\frac{q_3}{q_{\tau_{\max}}}I & \dots & -\frac{q_{\tau_{\max}-1}}{q_{\tau_{\max}}}I
\end{bmatrix}M
\end{align}
where $M$ is a block Toeplitz matrix as follows
\begin{align}
M=
\begin{bmatrix}
	\Sigma_{X_{\tau_{\max}+1}} & \Sigma_{X_{\tau_{\max}+2}} & \dots & \Sigma_{X_{2\tau_{\max}+1}} \\
	\Sigma_{X_{\tau_{\max}}} & \Sigma_{X_{\tau_{\max}+1}} & \dots & \Sigma_{X_{2\tau_{\max}}} \\
	\vdots & \vdots & \ddots & \vdots \\
	\Sigma_{X_{1}} & \Sigma_{X_{2}} & \dots & \Sigma_{X_{\tau_{\max}+1}}
\end{bmatrix}.
\end{align}

\begin{lem}\label{lm:inst}
	There is an instance of parameters for which matrix $M$ is full-rank.
\end{lem}
\begin{proof}
Let $A=D=0$, $B=bI, 0<b<1$, $Q$ being a uniform distribution in $[0 \; , \; \tau_{\max}]$, $\Sigma_V=0$ and $\Sigma_W=I$. Therefore, we have 
\begin{align}\label{eq:ins}
x_t=bx_{t-\tau-1}+w_t.
\end{align}
Since variables are independent with the same distribution, all matrices $\Sigma_{X_i}, i\in [1 \;, \; 2\tau_{\max}+1],$ are multiples of identity. Therefore, we can write $M=M_1 \otimes I$, where $M_1$ is the corresponding matrix for one variable, as follows
\begin{align}
M_1=
\begin{bmatrix}
\sigma_{X_{\tau_{\max}+1}} & \sigma_{X_{\tau_{\max}+2}} & \dots & \sigma_{X_{2\tau_{\max}+1}} \\
\sigma_{X_{\tau_{\max}}} & \sigma_{X_{\tau_{\max}+1}} & \dots & \sigma_{X_{2\tau_{\max}}} \\
\vdots & \vdots & \ddots & \vdots \\
\sigma_{X_{1}} & \sigma_{X_{2}} & \dots & \sigma_{X_{\tau_{\max}+1}}
\end{bmatrix}.
\end{align}
where $\sigma$ denotes the covariance of one variable. Since $\mathrm{rank}(M)=p \; \mathrm{rank}(M_1)$, we only need to show that matrix $M_1$ is full-rank.

Let $q=\frac{1}{\tau_{\max}+1}$. Using Equ.~\ref{eq:ins}, we can write
\begin{align}\label{eq:ins2}
\begin{cases}
\sigma_{X}=bq\sum_{j=0}^{\tau_{\max}}\sigma_{X_{j+1}}+1 \\
\sigma_{X_i}=bq\sum_{j=0}^{\tau_{\max}}\sigma_{X_{j+1-i}}, 1 \leq i \leq \tau_{\max}+1.
\end{cases}
\end{align}
By solving the system of equations in \ref{eq:ins2}, we have
\begin{align}\label{eq:ins3}
\begin{cases}
\sigma_{X}=\frac{(1-b)\tau_{\max}+1}{(1-b)\tau_{\max}+(1-b^2)} \\
\sigma_{X_i}=\frac{b}{(1-b)\tau_{\max}+(1-b^2)}, 1 \leq i \leq \tau_{\max}+1.
\end{cases}
\end{align}

Also, using the following equation
\begin{align}\label{eq_ins}
\begin{bmatrix}
\sigma_{X_{0}} & \sigma_{X_{1}} & \dots & \sigma_{X_{\tau_{\max}}}
\end{bmatrix}=
\begin{bmatrix}
\frac{b^{-1}}{q} & -1 & -1 & \dots & -1
\end{bmatrix}M_1,
\end{align}
we can solve $\sigma_{X_{\tau_{\max}+2}}=b\sigma_{X_{\tau_{\max}+1}}$, and since $b<1$, therefore $\sigma_{X_{\tau_{\max}+2}}\neq \sigma_{X_{\tau_{\max}+1}}$. Now, we compute the determinant of $M_1$ by doing the matrix column operation. More specifically, we replace $m_i$  with $m_i-m_{i+1},1 \leq i \leq \tau_{\max},$ where $m_i$ is the $i$-th column of $M_1$. The new matrix is an upper triangular matrix, as follows
\begin{align}
M'_1=
\begin{bmatrix}
\sigma_{X_{\tau_{\max}+1}}-\sigma_{X_{\tau_{\max}+2}} & \sigma_{X_{\tau_{\max}+2}}-\sigma_{X_{\tau_{\max}+3}} & \dots & \sigma_{X_{2\tau_{\max}}}-\sigma_{X_{2\tau_{\max}+1}} & \sigma_{X_{2\tau_{\max}+1}} \\
0 & \sigma_{X_{\tau_{\max}+1}}-\sigma_{X_{\tau_{\max}+2}} & \dots & \sigma_{X_{2\tau_{\max}-1}}-\sigma_{X_{2\tau_{\max}}} & \sigma_{X_{2\tau_{\max}}} \\
\vdots & \vdots & \ddots & \vdots & \vdots \\
0 & 0 & \dots & \sigma_{X_{\tau_{\max}+1}}-\sigma_{X_{\tau_{\max}+2}} & \sigma_{X_{\tau_{\max}+2}} \\
0 & 0 & \dots & 0 & \sigma_{X_{\tau_{\max}+1}}
\end{bmatrix}.
\end{align}
Since all diagonals are nonzero, the determinant of $M'_1$ is nonzero, and, as a result, matrix $M'_1$ and also $M_1$ are full-rank.
\end{proof}

\begin{lem}
	The set of zeros of any nonzero multivarite polynomial of degree $n$ has Lebesgue measure zero on $\mathbb{R}^n$.\label{lm:lebes}\cite{geiger2015causal}
\end{lem}

\begin{thm}
	Matrix $M$ is full-rank, with probability one.
\end{thm}
\begin{proof}
According to Lemma~\ref{lm:VX}, each entry of $\Sigma_{X_i}$ can be written as a rational function, where both the nominator and the denominator are multivariate polynomials in entries of the system parameters $A$, $B$, $D$, $Q$, $\Sigma_V$ and $\Sigma_W$. Therefore, we can conclude that $\det(M)=\frac{P}{Q}$, where $P$ and $Q$ are multivariate polynomials in entries of the system parameters. 
According to Lemma~\ref{lm:inst}, these multivarite polynomials are nonzero, because there exists an instance which results in a nonzero value for $\det(M)$. Since the Lebesgue measure of roots of a nonzero multivariate polynomial is zero, we conclude that $\det(M)$ is nonzero with probability one.
\end{proof}

\begin{thm}
	Matrix $M$ is full-rank for $\tau'<\tau_{\max}$, with probability one, and is not full-rank for $\tau'>\tau_{\max}$.
\end{thm}
\begin{proof}
	Therefore, we can find $\tau_{\max}$ as the maximum value for which matrix $M$ is full-rank.
\end{proof}

Now, we are ready to prove Theorem~\ref{thm:param}. Consider Equ.~\ref{Eq:identif}, Since $M$ is full-rank, we can obtain the parameters $\frac{B^{-1}}{q_{\tau_{\max}}}$, $\frac{q_0I+K_1}{q_{\tau_{\max}}}$, $\frac{q_1I - K_2}{q_{\tau_{\max}}}$ and $\frac{q_i}{q_{\tau_{\max}}}, 2 \leq i \leq \tau_{\max}-1$. Recall that $K_1=B^{-1}(A+D)$ and $K_2=B^{-1}AD$. We have the following results for identifiability.
\begin{itemize}
	\item If the PDF of $\tau$ is known, then we can identify $B$, $L_1=A+D$ and $L_2=AD$. In case that $D$ is diagonal, it can be identified by comparing the off-diagonal entries of $L_1$ and $L_2$. As a result, $A$ can also identified. 
	\item If the PDF of $\tau$ is not known, then we can identify $B$ up to a scale. In case that $B$ and $D$ are diagonal, by comparing the off-diagonal entries of $\frac{q_0I+K_1}{q_{\tau_{\max}}}$ and $\frac{q_1I - K_2}{q_{\tau_{\max}}}$, we can identify $D$ and also the off-diagonal entries of $A$.
\end{itemize}
